# Supplementary material for: Line lasing in a two-dimensional lattice of orbital photonic resonators
Source: arXiv:2512.18719 ancillary file (2026-07-02)
Supplement: Supplementary file 1 [file Line_lasing_Supplemental.pdf]

# Line lasing in a two-dimensional lattice of orbital photonic resonators: Supplemental Material

## 1. EXPERIMENTAL SCHEME

Figure S1 illustrates the experimental setup. The sample consists of a Lieb *sp* lattice placed inside a vacuum within a closed cycle helium cryostat and maintained at a temperature of 4 K, as recorded at the sample holder. A narrow linewidth ( $<10\text{MHz}$ ) single-mode Ti:Sapphire laser serves as the excitation source (wavelength  $820\text{nm}$ ). The beam is delivered through a single mode polarization maintaining optical fiber to ensure a high quality Gaussian spatial profile. After exiting the fiber, the beam power is regulated using a combination of a half-wave plate ( $\lambda/2$ ) and a polarizing beam splitter (PBS), which together serve as a tunable power control unit. To generate two different excitation spots we divide the excitation beam in using a beamsplitter. Each arm is equipped with a cylindrical lens (focal length  $f = 700\text{ mm}$ ) to create elongated Gaussian spots independently in each arm. The beams are then recombined at a PBS, forming the final excitation profile. A portion of the beam is diverted by a beam splitter (BS) for power monitoring, while the rest is directed toward the sample for excitation. A portion of the beam is diverted by a beam splitter (BS) for power monitoring, while the rest is directed toward the sample for excitation.

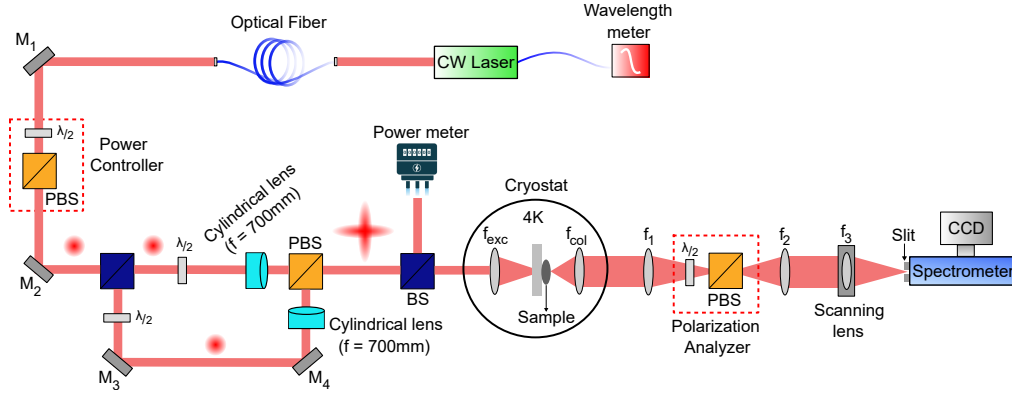

**Fig. S1.** Scheme of the experimental setup illustrating the excitation of the Lieb *sp* lattice and real space imaging of polariton photoluminescence (PL). Abbreviations:  $\frac{\lambda}{2}$  - half-wave retarder, PBS - polarized beam splitter, BS - beam splitter. Lenses:  $f_{exc}, f_{col} = 8\text{ mm}$ ,  $f_1 = 300\text{ mm}$ ,  $f_2 = 150\text{ mm}$  and  $f_3 = 500\text{ mm}$ .

The measurements are carried out in a transmission geometry: the excitation beams enter the sample through the epitaxial side, propagate through the substrate, and exit via a 3mm slit in the sample holder before reaching the collection optics. Both excitation and detection optics employ aspheric lenses ( $f_{exc}, f_{col}$ ) with a numerical aperture of 0.5. It is worth noting that the GaAs substrate exhibits negligible absorption at the operating wavelength allowing efficient light transmission. The photoluminescence emitted from the sample is first magnified using a telescope composed of two lenses with focal lengths  $f_1$  and  $f_2$ . Following this, the beam passes through a polarization analysis setup consisting of a half-wave plate ( $\lambda/2$ ) and a polarizing beam splitter (PBS). The transmitted light is then collected by a scanning objective lens ( $f_3$ ) and directed either to a CCD camera for imaging or to a spectrometer for spectral analysis. For Fourier space imaging, an additional lens is inserted between the telescope and the scanning lens.

## 2. LINE LASING IN A $10 \times 10$ LATTICE

In the main manuscript, the experimental results were presented for a  $4 \times 4$  lattice configuration. To demonstrate that the observed line lasing behavior and polarization locking phenomena are

not specific to the system size, here we present measurements performed on a larger  $10 \times 10$  lattice etched in the same microcavity wafer.

Real space imaging of the polariton photoluminescence was performed at the top of the  $sp$  band under a horizontally elongated excitation spot. All panels in Fig. S2(a) were taken above the lasing threshold, with a pump power of 35 mW. The emission was recorded for four linear output polarization angles:  $135^\circ$ ,  $0^\circ$ ,  $45^\circ$ , and  $90^\circ$ , corresponding to distinct analyzer orientations. In Fig. S2(b), a similar set of measurements was carried out using a vertically elongated excitation spot, also pumped above threshold at 35 mW. Real space images were recorded under the same set of output polarization angles ( $135^\circ$ ,  $0^\circ$ ,  $45^\circ$ , and  $90^\circ$ ). In the cross-pump excitation configuration as shown in Fig. S2(c), real space emission was again recorded under the four linear analyzer angles at a combined total power of 71 mW.

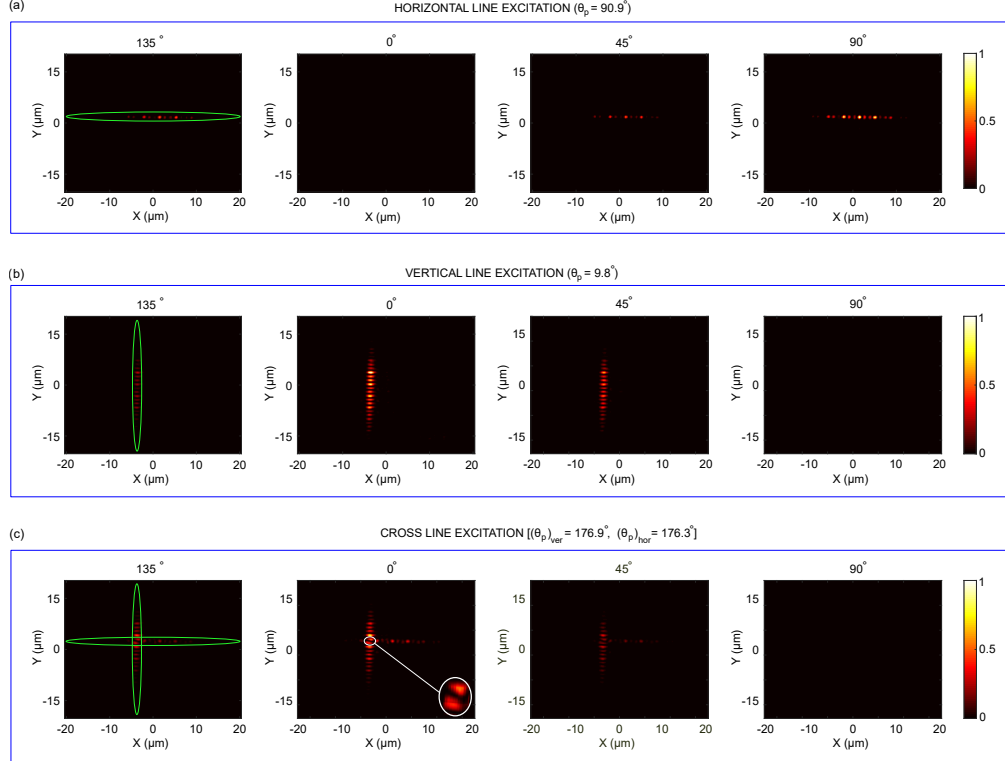

**Fig. S2.** Real space photoluminescence (PL) images analyzed at four output polarization angles:  $135^\circ$ ,  $0^\circ$ ,  $45^\circ$ , and  $90^\circ$ , using a polarization analyzer consisting of a half-wave plate and linear polarizer. (a) PL from the horizontal line with horizontal spot excitation at  $P = 35$  mW. (b) PL from the vertical line with vertical spot excitation at  $P = 35$  mW. (c) PL under cross pumping excitation with a total power of 71 mW. All images are extracted at a fixed energy slice (top  $sp$  band).

To extract the orientation of linear polarization from the measured photoluminescence for above three cases, intensities obtained by integrating the PL signal along a fixed energy (top of  $sp$  band) is calculated at four linear polarization analyzer angles:  $135^\circ$ ,  $0^\circ$ ,  $45^\circ$ , and  $90^\circ$  respectively. The Stokes parameters  $S_0$ ,  $S_1$ , and  $S_2$  were calculated using the following relations:

$$S_0 = I_{0^\circ} + I_{90^\circ} \quad (S1)$$

$$S_1 = I_{0^\circ} - I_{90^\circ} \quad (S2)$$

$$S_2 = I_{45^\circ} - I_{135^\circ} \quad (S3)$$

$$S_3 = 0 \quad (\text{assuming negligible circular polarization}) \quad (S4)$$

The angle of linear polarization is calculated using:

$$\theta_p = \frac{1}{2} \tan^{-1} \left( \frac{S_2}{S_1} \right) \quad (S5)$$

The computed angle  $\theta_p$  gives the polarization of the line lasing mode. For horizontal excitation,  $\theta_p = 90.9^\circ$  (vertical polarization), while for vertical excitation,  $\theta_p = 9.8^\circ$  (horizontal polarization). Under cross-pump conditions, the vertical line yields  $(\theta_p)_{\text{ver}} = 176.9^\circ$  (horizontally polarized) and the horizontal line gives  $(\theta_p)_{\text{hor}} = 176.3^\circ$  (horizontally polarized). These results confirm that the two line modes are both phase (as shown in the inset of Fig. S2(c)) and polarization locked, consistent with the behavior observed in the  $4 \times 4$  lattice.

Note that the power arrangement between the two pump spots shown in the main paper with a  $4 \times 4$  lattice resulted in vertical polarization locking. In the experiments displayed in Fig. S2 for a  $10 \times 10$  lattice the two spots have slightly different powers ( $P_{\text{horarm}} = 38$  mW and  $P_{\text{verarm}} = 33$  mW) such that the local blueshifts result in an energy degeneracy of modes with horizontal polarization.

### 3. INTERFERENCE EXPERIMENT

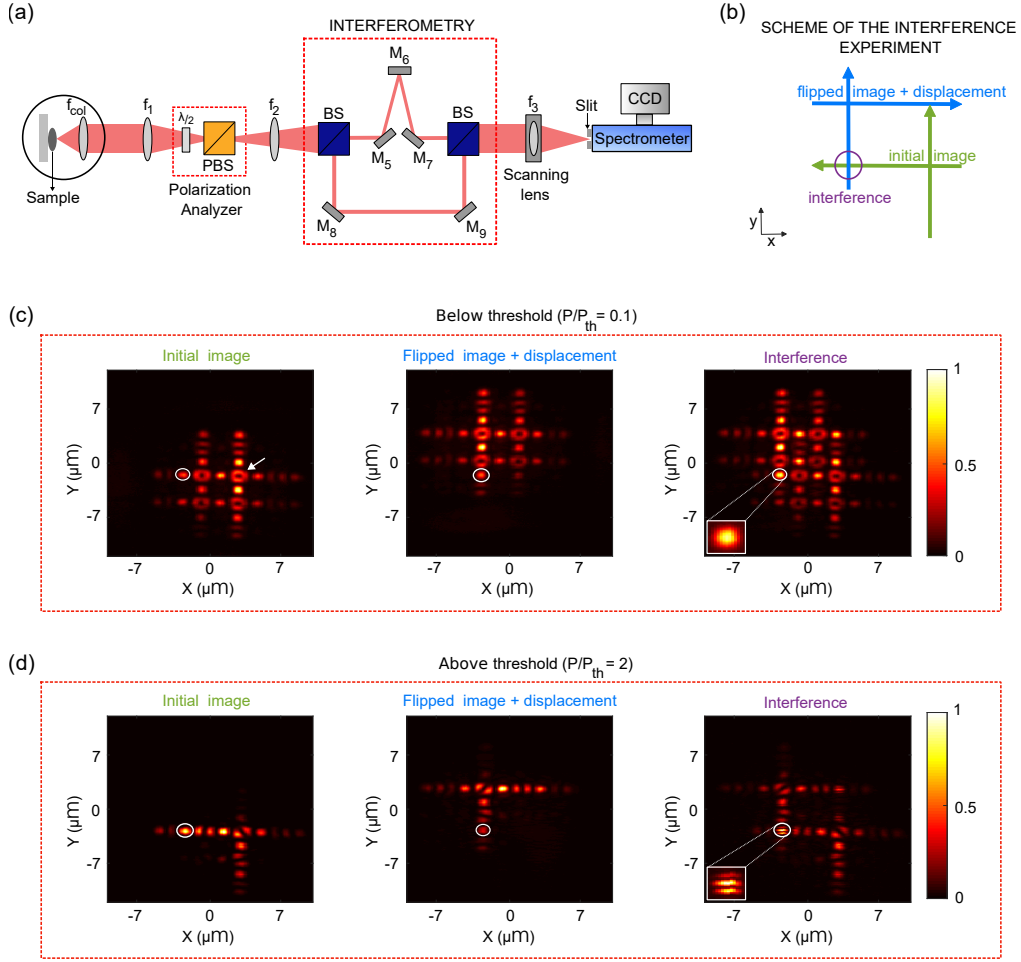

**Fig. S3.** (a) Schematic of the experimental setup for the interferometry. (b) Illustration of the interference procedure: the initial image is flipped and spatially displaced then recombined to produce the interference pattern. (c) Interferogram recorded below threshold power, where no interference is observed (shown as an inset). (d) Interferogram recorded above the threshold power, revealing clear interference fringes (shown as an inset).

To confirm the phase locking of the two orthogonal line modes, an interferometric measurement was performed. Fig. S3(a) shows the interferometer configuration using three mirrors, with mirror  $M_6$  mounted on a kinematic stage for fine adjustment. This allows precise control of the optical path length to achieve near zero delay between the two arms, which is essential for observing interference and verifying phase coherence between the modes.

Figure S3(b) illustrates the schematic of the interference process. One arm of the interferometer captures the direct image of the emission, while the other arm produces a spatially displaced and mirror-flipped version of the same image. This configuration allows the two images to overlap and interfere.

Figure S3(c) - left panel- shows the initial image below threshold. Emission is spread over several lines in the lattice. At the crossing site of the two pump spots (see arrow), we observe a ring like emission. This ring pattern is characteristic of the random phase between the  $p_x$  and  $p_y$  orbitals in the spontaneous emission regime below threshold. The white circles in the left and central images of Fig. S3(c) highlight the spatial regions where the  $s$ -orbital modes from the two orthogonal lines are made to interfere in the right panel. The absence of interference fringes witnesses the absence of phase locking in the spontaneous emission regime at  $P/P_{th} = 0.1$ . Above threshold ( $P/P_{th} = 2$ ), Fig. S3(d) shows the emergence of interference fringes, clearly visible in the inset of the right panel, indicating phase locking.

#### 4. POLARIZATION RESOLVED EMISSION

In this section we provide additional experimental details on the polarization resolved emission for the crossed lines excitation. We focus on the conditions described in the main text for the crossed lines excitation of a  $4 \times 4$  lattice reported in Fig. 5.

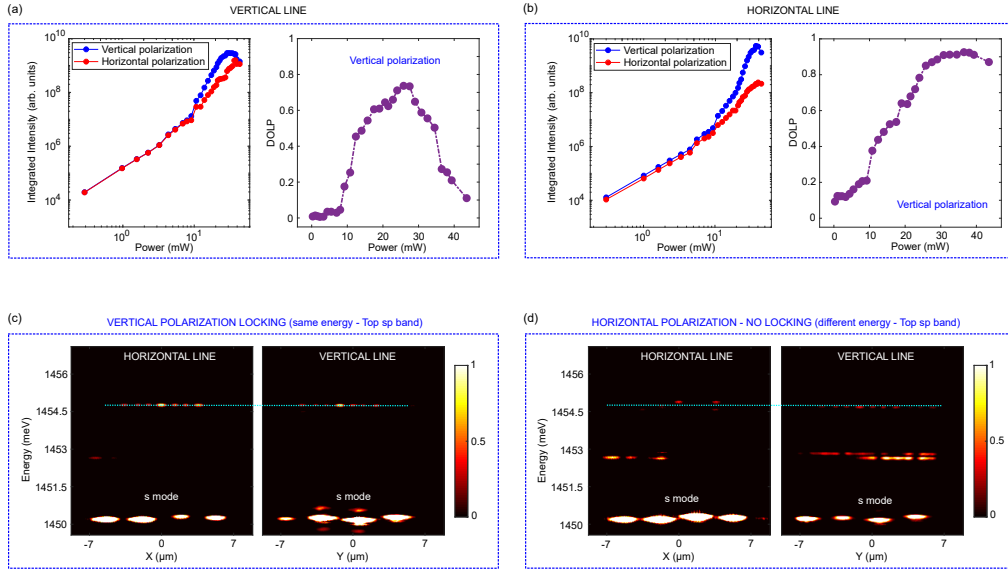

**Fig. S4.** (a) Integrated intensity of the upper  $sp$  mode along the vertical line for a cross pumping configuration in which the lattice is excited. The intensity is resolved in linear polarization and the Degree of linear polarization (DOLP) is computed from the integrated intensity. b) Integrated intensity of the upper  $sp$  mode along the horizontal line for a cross pumping configuration in which the lattice is excited. The intensity is resolved in linear polarization and the Degree of linear polarization (DOLP) is computed from the integrated intensity. c) Polarization locking observed due to the degeneracy of the top  $sp$  band for both the vertical and horizontal line. d) Absence of polarization locking, attributed to the energy difference between the top  $sp$  bands along the vertical and horizontal line.

Figures S4(a) and (b) display the polarization resolved emission integrated spatially over each of excited lines (vertical line in (a), horizontal line in (b)) at the energy of the top of the  $sp$  bands. The horizontal axis corresponds to the total excitation power (sum of the power of the two spots). Above threshold, the degree of linear vertical polarization is high for both lines.

In the main text of Fig. 5(c) analysis of blueshift was done at  $P/P_{th} = 1.2$ . As an additional proof, Fig. S4(c) shows the energy spectra of the emission along the vertical and horizontal lasing lines with the analyzer in the vertical linear polarization position, which corresponds to the polarization of the laser emission, for an excitation power well above threshold ( $P/P_{th} = 1.6$ ). The laser emission energy in this polarization for the modes at the top of the  $sp$  bands is identical

up to our spectral resolution (dashed line). Figure S4(d) shows the energy spectra of the emission with opposite polarization (horizontal), for the two lasing lines. Emission from the top of the  $sp$  bands is weaker but still visible. However, it does not happen at the energy of the vertical polarization emission of the lasing mode in Fig. S4(c). Each line of the lattice emits horizontally polarized light at the top of the  $sp$  band at different energies. This polarization behavior is displayed in Fig. 5(d) of the main text. It shows that different blueshifts on each line are required for polarization alignment and locking of the lasing mode.
